# Supplementary material for: Cooperative quantum interface for noise mitigation in quantum networks
Source: arXiv:2411.13158 source file (2024-11-20)
Supplement: Supplementary file 1 [file SM3.pdf]

# Supplemental Material for "Cooperative quantum interface for noise mitigation in quantum networks"

Yan-Lei Zhang,[1,2,*] Ming Li,[1,2,*] Xin-Biao Xu,[1,2] Chun-Hua Dong,[1,2,3] Guang-Can Guo,[1,2,3] Ze-Liang Xiang,[4,†] Chang-Ling Zou,[1,2,3,‡] and Xu-Bo Zou[1,2,3,§]

[1]*Key Laboratory of Quantum Information, CAS, University of Science and Technology of China, Hefei 230026, China*

[2]*CAS Center For Excellence in Quantum Information and Quantum Physics, University of Science and Technology of China, Hefei, Anhui 230026, P. R. China*

[3]*Hefei National Laboratory, University of Science and Technology of China, Hefei 230088, China.*

[4]*School of Physics, Sun Yat-sen University, Guangzhou 510275, China.*

(Dated: September 16, 2024)

## CONTENTS

I. Model S1
  A. The cooperative quantum interface (CQI) S1
  B. The traditional cascaded (CAS) system S2

II. Entanglement of two remote nodes S3

III. Cooperative effect against thermal noise S6

IV. Entanglement of multiple remote nodes S7

V. Quantitative analysis of experimental feasibility S7

VI. The fidelity for the input pulsed light S8

References S9

## I. MODEL

### A. The cooperative quantum interface (CQI)

Two coupled optical modes based on the frequency conversion (FC), realized by the pump driving laser with the frequency $\omega_d$, and one qubit coupled to alternative optical mode, constitute a hybrid system, where the corresponding coupling strengths are $G$ and $\mu$, respectively. Including the external continuous optical field and the decay rates of optical modes and the qubit, we can obtain the full Hamiltonian of the hybrid system as ($\hbar = 1$ and $c = 1$) [1–3]:

$$\begin{aligned} H_{\rm sys} &= \omega_a a^\dagger a + \Delta_b b^\dagger b + \Delta_q \left|e\right\rangle\left\langle e\right| + G\left(a^\dagger b + a b^\dagger\right) + \mu\left(\sigma_+ b + \sigma_- b^\dagger\right) + i\sqrt{\kappa_{a,ex}}\left(c_0 a^\dagger - c_0^\dagger a\right) \\ &+ \frac{i}{2}\int_{-\infty}^{\infty}\left[\partial_x\left(c_x^\dagger\right)c_x - c_x^\dagger\partial_x\left(c_x\right)\right]dx - \frac{i}{2}\kappa_{a,o}a^\dagger a - \frac{i}{2}\kappa_{b,o}b^\dagger b - \frac{i}{2}\gamma\left|e\right\rangle\left\langle e\right|, \end{aligned} \tag{S.1}$$

where $\Delta_b = \omega_b - \omega_d$ and $\Delta_q = \omega_{eg} - \omega_d$; $\omega_{a(b)}$ and $\omega_{eg}$ are frequencies of optical modes and the qubit; $\kappa_{a,o}$ ($\kappa_{b,o}$), and $\gamma$ are the dissipation rates of optical modes $a\,(b)$ and the qubit; $c_x$ is the external continous optical field in the real space; $\kappa_{a,ex}$ is the coupling strength between the optical mode $a$ and the external field $c_0$. Here the optical mode $b$ has no interaction with the external field, and it acts as a bridge to provide a channel between the mode $a$ and the qubit.

---

* These two authors contributed equally to this work.
† xiangzliang@mail.sysu.edu.cn
‡ clzou321@ustc.edu.cn
§ xbz@ustc.edu.cn

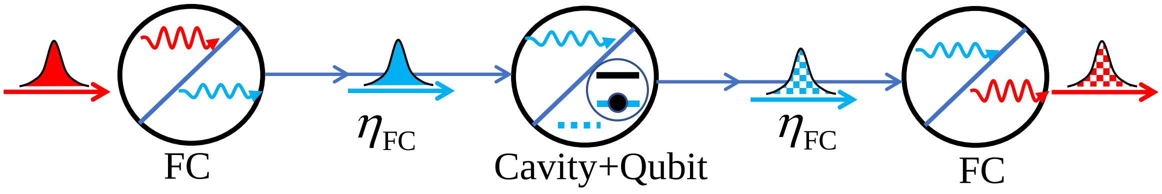


FIG. S1. Schematic diagram of the traditional cascaded system. FC: Frequency conversion. $\eta_{\mathrm{FC}}$ is the FC efficiency.

For the single-photon problem, a general state $|\Psi(t)\rangle$ can be expanded in the single-excitation subspace as

$$\begin{aligned}|\Psi(t)\rangle &= \int_{-\infty}^{\infty} f(x,t)|x\rangle_{ex}|0\rangle_a|0\rangle_b|g\rangle dx + \Phi_a(t)|\emptyset\rangle_{ex}|1\rangle_a|0\rangle_b|g\rangle + \Phi_b(t)|\emptyset\rangle_{ex}|0\rangle_a|1\rangle_b|g\rangle \\ &+\lambda_e(t)|\emptyset\rangle_{ex}|0\rangle_a|0\rangle_b|e\rangle, \end{aligned} \tag{S.2}$$

where $f(x,t)$ is the complex amplitude of the external field in the $x$ location, $|\emptyset\rangle_{ex}$ is the external vacuum state, $\Phi_{a(b)}(t)$ is the complex amplitude in the state $|1\rangle_{a(b)}$, and $\lambda_e(t)$ is the probability amplitude of the qubit in the excited state.

The dynamics of the system is governed by the equation $i\frac{\partial}{\partial t}|\Psi(t)\rangle = H_{sys}|\Psi(t)\rangle$, and we obtain the following equations of motion:

$$i\frac{\partial f(x,t)}{\partial t} = -i\frac{\partial f(x,t)}{\partial x} - i\sqrt{\kappa_{a,ex}}\Phi_a(t)\delta(x), \tag{S.3}$$

$$\begin{aligned} i\frac{\partial \Phi_a(t)}{\partial t} &= \left(\omega_a - \frac{i}{2}\kappa_a\right)\Phi_a(t) + G\Phi_b(t) + i\sqrt{\kappa_{a,ex}}f(0-,t), \\ i\frac{\partial \Phi_b(t)}{\partial t} &= \left(\Delta_b - \frac{i}{2}\kappa_{b,o}\right)\Phi_b(t) + G\Phi_a(t) + \mu\lambda_e(t), \\ i\frac{\partial \lambda_e(t)}{\partial t} &= \left(\Delta_q - \frac{i\gamma}{2}\right)\lambda_e(t) + \mu\Phi_b(t). \end{aligned} \tag{S.4}$$

Here $x<0$ ( $x>0$ ) represents the input (output) field, and we have assumed $f(0,t) = [f(0+,t) + f(0-,t)]/2$. From the equation S.3, we have $f(0+,t) - f(0-,t) = -\sqrt{\kappa_{a,ex}}\Phi_a(t)$, where $f(0-,t)$ is the input single photon. In fact, we know that the general general condition is that the length of the pulse satisfies $\tau \gg \kappa_a, \kappa_{b,o}$, which can be regarded as a continuous light. In the frequency space, we can obtain the results

$$\Phi_a = \frac{-i\sqrt{\kappa_{a,ex}}}{(\omega_a-\omega) - \frac{i\kappa_a}{2} - \frac{G^2}{(\Delta_b-\omega)-\frac{i}{2}\kappa_{b,o}-\mu^2/[(\Delta_q-\omega)-i\gamma/2]}}, \tag{S.5}$$

$$f_u = \frac{(\omega_a-\omega) - \frac{i\kappa_a}{2} - \frac{G^2}{(\Delta_b-\omega)-\frac{i}{2}\kappa_{b,o}-\mu^2/[(\Delta_q-\omega)-i\gamma/2]} + i\kappa_{a,ex}}{(\omega_a-\omega) - \frac{i\kappa_a}{2} - \frac{G^2}{(\Delta_b-\omega)-\frac{i}{2}\kappa_{b,o}-\mu^2/[(\Delta_q-\omega)-i\gamma/2]}}, \tag{S.6}$$

where $f_u$ is the output photon and $\kappa_a = \kappa_{a,ex} + \kappa_{a,o}$.

### B. The traditional cascaded (CAS) system

The traditional cascaded system is shown in Fig. S1, and the whole process is decomposed as the frequency conversion (FC)$\rightarrow$functional device (Cavity+Qubit) $\rightarrow$frequency conversion (FC), which bring in the additional

insertion loss that means $\eta_{\mathrm{FC}} < 1$. The corresponding to the Hamiltonian is

$$\begin{aligned} H_{\mathrm{FC}} &= \omega_a a^\dagger a + \Delta_b b_1^\dagger b_1 + G\left(a^\dagger b_1 + a b_1^\dagger\right) + i\sqrt{\kappa_{a,ex}}\left(c_0 a^\dagger - c_0^\dagger a\right) + i\sqrt{\kappa_{b,ex}}\left(c_0 b_1^\dagger - c_0^\dagger b_1\right) \\ &+\frac{i}{2}\int_{-\infty}^{\infty}\left[\partial_x\left(c_x^\dagger\right)c_x - c_x^\dagger \partial_x\left(c_x\right)\right]dx - \frac{i}{2}\kappa_{a,o}a^\dagger a - \frac{i}{2}\kappa_{b,o}b_1^\dagger b_1, \qquad \text{(S.7)} \\ H_{\mathrm{I}} &= \Delta_b b_2^\dagger b_2 + \Delta_q \left|e\right\rangle\left\langle e\right| + \mu\left(\sigma_+ b_2 + \sigma_- b_2^\dagger\right) + i\sqrt{\kappa_{b,ex}}\left(c_0 b_2^\dagger - c_0^\dagger b_2\right) \\ &-\frac{i}{2}\kappa_{b,o}b_2^\dagger b_2 - \frac{i}{2}\gamma\left|e\right\rangle\left\langle e\right|, \qquad \text{(S.8)} \end{aligned}$$

where $\kappa_{b,ex}$ is the external coupling rate of the mode $b_1\,(b_2)$ and we assume that the parameters about the mode $b_1\,(b_2)$ are same for the $H_{\mathrm{FC}}$ and $H_{\mathrm{I}}$.

For the FC process, we obtain the conversion efficiency

$$\eta_{\mathrm{FC}} = \frac{G^2\kappa_{b,ex}\kappa_{a,ex}}{\left|\Delta_b - \omega - \frac{i}{2}\kappa_b\right|^2\left|(\omega_a-\omega) - \frac{i\kappa_a}{2} - \frac{G^2}{(\Delta_b-\omega)-\frac{i}{2}\kappa_b}\right|^2}, \qquad \text{(S.9)}$$

where $\kappa_b = \kappa_{b,ex} + \kappa_{b,o}$. We know $\eta_{\mathrm{FC}} \leq 1$ for $\kappa_{b,ex} \leq \kappa_b$ and $\kappa_{a,ex} \leq \kappa_a$. For the functional device, we assume that the general sate in the single-excitation subspace can be written as

$$\left|\Psi(t)\right\rangle = \int_{-\infty}^{\infty} f(x,t)\left|x\right\rangle_{ex}\left|0\right\rangle_b\left|g\right\rangle dx + \Phi_b(t)\left|\emptyset\right\rangle_{ex}\left|1\right\rangle_b\left|g\right\rangle + \lambda_e(t)\left|\emptyset\right\rangle_{ex}\left|0\right\rangle_b\left|e\right\rangle, \qquad \text{(S.10)}$$

and the corresponding dynamical equations are

$$\begin{aligned} i\frac{\partial f(x,t)}{\partial t} &= -i\frac{\partial f(x,t)}{\partial x} - i\sqrt{\kappa_{b,ex}}\Phi_b(t)\delta(x), \qquad \text{(S.11)} \\ i\frac{\partial \Phi_b(t)}{\partial t} &= \left(\Delta_b - \frac{i}{2}\kappa_{b,0}\right)\Phi_b(t) + \mu\lambda_e(t) + i\sqrt{\kappa_{b,ex}}f(0,t), \qquad \text{(S.12)} \\ i\frac{\partial \lambda_e(t)}{\partial t} &= \left(\Delta_q - \frac{i\gamma}{2}\right)\lambda_e(t) + \mu\Phi_b(t). \qquad \text{(S.13)} \end{aligned}$$

In the frequency space, the results are

$$\begin{aligned} \Phi_b &= \frac{-i\sqrt{\kappa_{b,ex}}}{(\Delta_b-\omega) - \frac{i\kappa_b}{2} - \frac{\mu^2}{(\Delta_q-\omega)-i\gamma/2}}, \qquad \text{(S.14)} \\ f_u &= \frac{(\Delta_b-\omega) - \frac{i\kappa_b}{2} - \frac{\mu^2}{(\Delta_q-\omega)-i\gamma/2} + i\kappa_{b,ex}}{(\Delta_b-\omega) - \frac{i\kappa_b}{2} - \frac{\mu^2}{(\Delta_q-\omega)-i\gamma/2}}. \qquad \text{(S.15)} \end{aligned}$$

## II. ENTANGLEMENT OF TWO REMOTE NODES

As shown in Fig. 2(a) in the manuscript, we use the beam splitter to realize the entanglement between two nodes. After the single photon passes through the first beam splitter, the photon state can be written as $\left(\left|\uparrow\right\rangle + i\left|\downarrow\right\rangle\right)/\sqrt{2}$, where the photon $\left|\uparrow\right\rangle$ and $\left|\downarrow\right\rangle$ interacts with the qubit 1 and 2, respectively. Meanwhile we prepare the initial qubit as $\left(\left|s\right\rangle + \left|g\right\rangle\right)/\sqrt{2}$, and the initial state is described as

$$\left|\Psi\right\rangle_0 = \frac{\left|\uparrow\right\rangle + i\left|\downarrow\right\rangle}{\sqrt{2}} \otimes \frac{\left|s\right\rangle_1 + \left|g\right\rangle_1}{\sqrt{2}} \otimes \frac{\left|s\right\rangle_2 + \left|g\right\rangle_2}{\sqrt{2}}, \qquad \text{(S.16)}$$

where $\left|s\right\rangle$ is the assisted state. When the qubit is in the state $\left|s\right\rangle$ or $\left|g\right\rangle$, the output photon acquires the opposite phase, which leads to the entanglement between the photon and the qubit. Through the second beam splitter, the

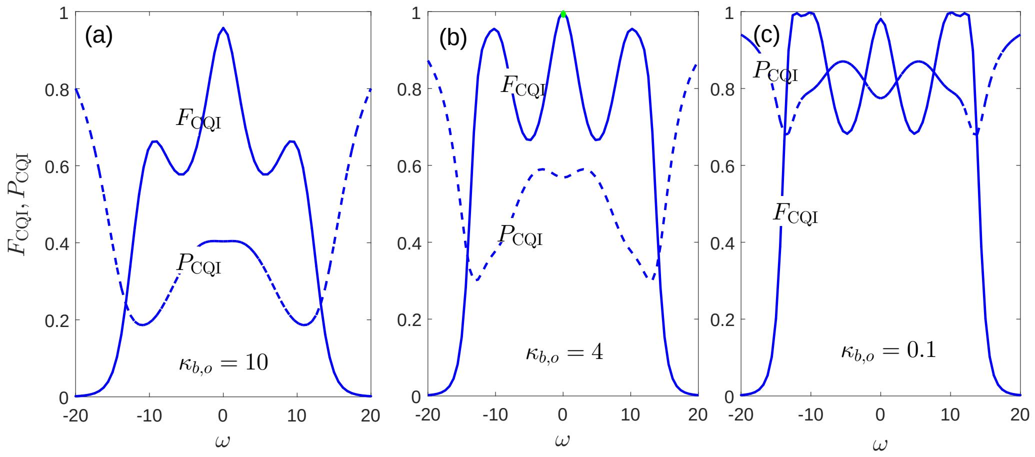


FIG. S2. The fidelity $F_{\rm CQI}$ and successful probability $P_{\rm CQI}$ as the function of the input photon frequency $\omega$ in the combined system for the different intrinsic loss $\kappa_{b,o}=10$ (a), 4 (b), 0.1 (c) from the intermediate mode $b$. Here we consider the resonant condition $\omega_a=\Delta_b=\Delta_q=0$, the other parameters are $\kappa_{a,o}=1$, $\kappa_{a,ex}=14$, $G=\mu=10$, and the qubit rate $\gamma$ is as a normalized unit. The green dot in Fig (b) is the ideal fidelity $F_{\rm CQI}=1$, which is corresponding to the intrinsic loss $\kappa_{b,o}=4$

ideal final state can be obtained

$$|\psi\rangle_{\rm ideal}=\frac{|+i\rangle}{2}\left(|s\rangle_1|s\rangle_2-|g\rangle_1|g\rangle_2\right)+\frac{|-i\rangle}{2}\left(|s\rangle_1|g\rangle_2-|g\rangle_1|s\rangle_2\right), \tag{S.17}$$

where $|+i\rangle=\frac{|\uparrow\rangle+i|\downarrow\rangle}{\sqrt{2}}$ and $|-i\rangle=\frac{|\uparrow\rangle-i|\downarrow\rangle}{\sqrt{2}}$. Here we have ignored the photon loss and other imperfections. If we measure the output photon state $|+i\rangle$ or $|-i\rangle$ by a single photon detector, the Bell state of two nodes is prepared. It means that we can realize the remote entanglement of two nodes as long as the photon is detected.

However, we have to consider all kinds of noises in practical experimental system. The real final state can be written as

$$\begin{aligned}|\Psi\rangle_f=&\frac{|+i\rangle}{2}\left[f_{\mu=0}|s\rangle_1|s\rangle_2+f_\mu|g\rangle_1|g\rangle_2+\frac{(f_{\mu=0}+f_\mu)}{2}\left(|s\rangle_1|g\rangle_2+|g\rangle_1|s\rangle_2\right)\right]\\&+\frac{|-i\rangle\,(f_{\mu=0}-f_\mu)}{4}\left(|s\rangle_1|g\rangle_2-|g\rangle_1|s\rangle_2\right),\end{aligned} \tag{S.18}$$

which is the ideal state $|\Psi\rangle_{\rm ideal}$ when $f_{\mu=0}=f_\mu=\pm1$. For the quantitative analysis of entanglement, we calculate the fidelity and the successful probability

$$\begin{aligned}F&=\frac{\left|\langle\Psi|_f\,|\Psi\rangle_{\rm ideal}\right|^2}{\langle\Psi|_f\,|\Psi\rangle_f}\\&=\frac{|f_{\mu=0}-f_\mu|^2}{2\left(|f_{\mu=0}|^2+|f_\mu|^2\right)},\end{aligned} \tag{S.19}$$

$$\begin{aligned}P&=\langle\Psi|_f\,|\Psi\rangle_f\\&=\frac{|f_{\mu=0}|^2+|f_\mu|^2}{2},\end{aligned} \tag{S.20}$$

where $F$ is the fidelity after the post selection.

The Fig. S2 shows the fidelity $F_{\rm CQI}$ and successful probability $P_{\rm CQI}$ as the function of the frequency $\omega$ for the

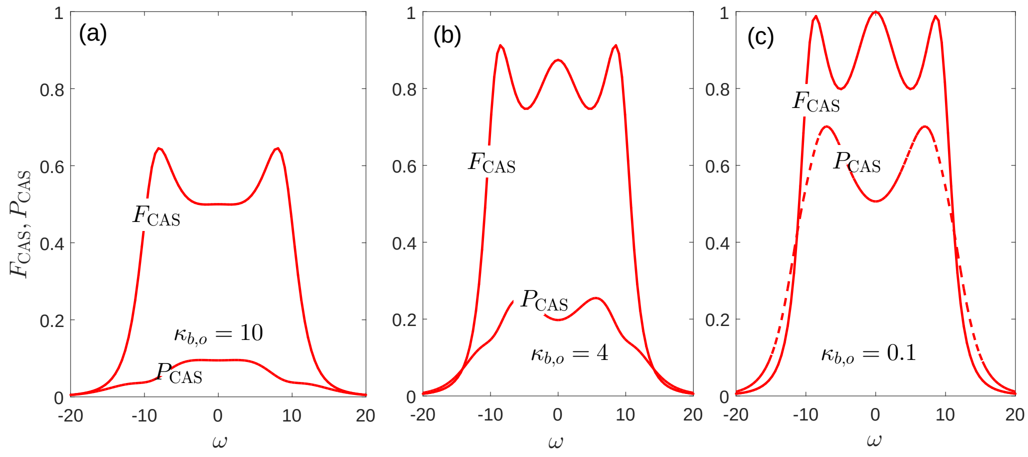


FIG. S3. The performance for the traditional cascaded system, where we introduce the external coupling rate $\kappa_{b,ex}=10$ and other parameters are the same as in Fig. S2.

different loss $\kappa_{b,o}=10$ (a), 4 (b), 0.1 (c). For the resonant condition that is $\omega=0$, we obtain the fidelity

$$F_{\rm CQI}=\frac{2\left|\frac{\kappa_{a,ex}C_{bq}C_{ab}}{\kappa_a(1+C_{ab})(1+C_{bq}+C_{ab})}\right|^2}{\left|1-\frac{2\kappa_{a,ex}}{\kappa_a(1+C_{ab})}\right|^2+\left|1-\frac{2\kappa_{a,ex}(1+C_{bq})}{\kappa_a(1+C_{bq}+C_{ab})}\right|^2}, \tag{S.21}$$

where $C_{b,q}=4\mu^2/(\gamma\kappa_{b,o})$ and $C_{a,b}=4G^2/(\kappa_a\kappa_{b,o})$ with $\kappa_{b,ex}=0$. These numerical results are in agreement with the analytical results. In addition, we also notice that there are two peaks for the fidelity except the resonant point, which are due to the interaction term $G\left(a^\dagger b+ab^\dagger\right)$. Therefore, we introduce the transformation $a=\cos\left(\frac{\theta}{2}\right)A+\sin\left(\frac{\theta}{2}\right)B$ and $b=-\sin\left(\frac{\theta}{2}\right)A+\cos\left(\frac{\theta}{2}\right)B$, and the corresponding frequencies of supermodes A and B are

$$\omega_A=\omega_a\cos^2\left(\frac{\theta}{2}\right)+\Delta_b\sin^2\left(\frac{\theta}{2}\right)-|G|\sin(\theta), \tag{S.22}$$

$$\omega_B=\Delta_b\cos^2\left(\frac{\theta}{2}\right)+\omega_a\sin^2\left(\frac{\theta}{2}\right)+|G|\sin(\theta), \tag{S.23}$$

where $\theta=\arctan\left(\frac{2|G|}{\Delta_b-\omega_a}\right)$. At the resonant condition $\omega_a=\Delta_b=0$, we apply the transformation $a=(A+B)/\sqrt{2}$ and $b=(B-A)/\sqrt{2}$ to diagonalize the interaction term, and the frequency of the supermode $A\,(B)$ is $\omega_A\,(\omega_B)=-G\,(G)$, which is corresponding to the peak of the fidelity. When the loss $R_{b,o}$ reduces, the cooperativity factors $C_{ab}$ and $C_{bq}$ will be increased, which leads to that the fidelity and efficiency are improved, as shown in Fig. S2(b). It is noticed that there exists a perfect point that makes the fidelity $F_{\rm CQI}=1$, which is the analogous impedance matching

$$\frac{1}{1+4G^2/(\kappa_a\kappa_{b,o})}+\frac{1+4\mu^2/(\gamma\kappa_{b,o})}{1+4\mu^2/(\gamma\kappa_{b,o})+4G^2/(\kappa_a\kappa_{b,o})}=\frac{\kappa_a}{\kappa_{a,ex}}. \tag{S.24}$$

If we ignore other noises, and the perfect fidelity is labeled as the green dot in Fig. S2(b). It means that the fidelity is weakened if we further decrease the loss $\kappa_{b,o}$, and the Fig. S2(c) illustrates exactly this point. It is interesting that the other two peaks show the better fidelity, which are close to the analogous impedance matching at the frequency $\omega=\omega_A\,(\omega_B)$. In conclusion, we can obtain the optimal fidelity by tuning the intermediate loss and the frequency of the input photon.

For the traditional cascaded system, we need to consider the conversion efficiency and the insertion loss. Therefore

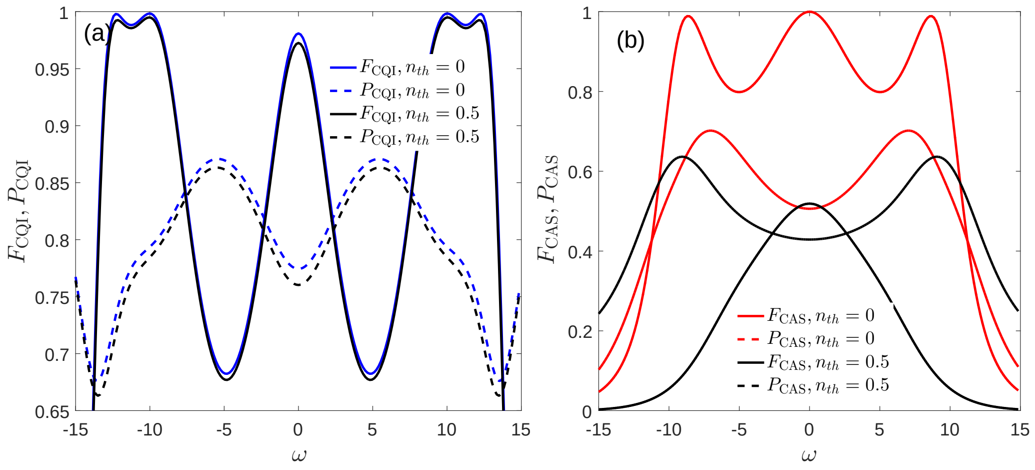


FIG. S4. The effect of thermal noise on the fidelity and the successful probability in the cooperative quantum interface system (a) and the cascaded system (b), where the intrinsic loss of the mode $b$ is $\kappa_{b,o}=0.1$ and other parameters are the same as in Fig. S3.

the final fidelity and successful probability are

$$F_{\rm CAS}=\frac{\left|f_{\mu=0}-f_{\mu}\right|^2}{2\left(\left|f_{\mu=0}\right|^2+\left|f_{\mu}\right|^2\right)}, \tag{S.25}$$

$$P_{\rm CAS}=\frac{\eta_{\rm FC}^2\left(\left|f_{\mu=0}\right|^2+\left|f_{\mu}\right|^2\right)}{2}, \tag{S.26}$$

where the $F_{\rm CAS}$ is the post selection fidelity, which has nothing to do with the conversion efficiency $\eta_{\rm FC}$. For the different loss $\kappa_{b,o}=10$ (a), 4 (b), 0.1 (c) in Fig. S3, the results show that the fidelity of the traditional cascaded system is lower than that of the combined system, especially for the large loss. When $\omega=0$, we have the fidelity

$$F_{\rm CAS}=\frac{2\left|\frac{\kappa_{b,ex}}{\kappa_b}-\frac{\kappa_{b,ex}}{\kappa_b(1+C_{bq})}\right|^2}{\left|1-\frac{2\kappa_{b,ex}}{\kappa_b}\right|^2+\left|1-\frac{2\kappa_{b,ex}}{\kappa_b(1+C_{bq})}\right|^2}, \tag{S.27}$$

where $C_{bq}=4\mu^2/(\gamma\kappa_b)$ with $\kappa_b=\kappa_{b,ex}+\kappa_{b,o}$. The efficiency is related to the FC efficiency

$$\eta_{\rm FC}=\frac{\kappa_{a,ex}}{\kappa_a}\frac{\kappa_{b,ex}}{\kappa_b}\frac{4C_{ab}}{(1+C_{ab})^2}, \tag{S.28}$$

where $C_{ab}=4G^2/(\kappa_a\kappa_b)$.

For the non-resonant case $\omega=\omega_A\,(\omega_B)$, the fidelity is better than the performance at the resonant condition, as shown in Fig. S3(a) and (b). It is rooted in the suppressive loss for the supermode $A\,(B)$ from the mode $b$ when the $\kappa_{b,o}$ is very large. However, these results are still worse than the performance in the combined system, which is due to the cooperative effect that can mitigate the loss from the intermediate mode.

## III. COOPERATIVE EFFECT AGAINST THERMAL NOISE

In addition to the vacuum loss $R_{b,o}$, the thermal noise is also one of the most important factors affecting the fidelity and successful probability in practical systems, especially for the FC that is from the communicate optical band to the microwave band or the phonon frequency. The mode $b$ is corresponding to the microwave mode or phonon mode, and the experimental system can be the superconducting system or solid system. The full system can be described

by the dynamic evolution equation of the density matrix

$$\frac{d\rho}{dt} = -i\left[H, \rho\right] + \kappa_a \mathcal{L}\left(a\right) + \gamma \mathcal{L}\left(\sigma_-\right) + \kappa_{b,o}\left(n_{th}+1\right)\mathcal{L}\left(b\right) + \kappa_{b,o} n_{th} \mathcal{L}\left(b^\dagger\right), \tag{S.29}$$

where $H$ is the Hamiltonian without the dissipative terms, the Lindblad super-operator $\mathcal{L}\left(o\right) = o\rho o^\dagger - \rho o^\dagger o/2 - o^\dagger o \rho/2$, and $n_{th}$ is the thermal noise from the mode $b$.

Here we use the weakly coherent light as the single photon input, and the output field is obtained after normalization. When $n_{th} = 0$ in Fig. S4, the results of numerical calculation by the above master equation are consistent with the analytical results in Fig. S2(c) and S3(c). In the case of thermal noise, it is obvious that there is no phase information for the photon converted from the thermal noise. Because we use the weakly coherent light as single photon source in the process of numerical calculation, the intracavity field $\langle a \rangle$ contains only the coherent photon, which has no thermal noise. We can obtain the thermal noise from the equation $\langle a^\dagger a \rangle - \left|\langle a \rangle\right|^2$, and therefore the fidelity and efficiency can be calculated numerically. The black lines in Fig. S4(a) show the the related results with $n_{th} = 0.5$, which show that the fidelity and efficiency are barely affected. Around the frequency $\omega = \omega_A \left(\omega_B\right)$, the thermal has the less effect than the resonant frequency $\omega = 0$, which is due to the cooperative effect. So we can obtain the optimal fidelity by tuning the driving frequency $\omega$.

As a contrast, we also calculate the cascaded system with the thermal noise in Fig. S4(b), and it is obvious that the fidelity and successful probability are seriously affected by the thermal noise, where we use the decay rate $\kappa_b$ instead of $\kappa_{b,o}$. Even if we have ignored the transmitting thermal noise of the cascaded system, the performance is far below the combined system. It is concluded that the comparison results show that the thermal noise is hugely suppressed, which can greatly improve the performance of the device, and we can obtain the optimal fidelity by adjusting the appropriate parameters.

## IV. ENTANGLEMENT OF MULTIPLE REMOTE NODES

Our scheme has more obvious advantages in constructing quantum networks, where we need to prepare the entanglement of of multiple remote nodes. So more FC devices are essential for the traditional cascaded system, while more insertion loss and noises are also introduced into the system, which greatly limits the expansion of nodes. Therefore, the cooperative effect in our scheme gives overwhelming advantages on expanding remote nodes to construct quantum networks.

Here we consider a simple extended multi-node scheme, and we first prepare two pairs of entangled states with two nodes, which are $\left|\Psi\right\rangle_{1,2} = \left(\left|s\right\rangle_1 \left|s\right\rangle_2 + \left|g\right\rangle_1 \left|g\right\rangle_2\right)/\sqrt{2}$ and $\left|\Psi\right\rangle_{3,4} = \left(\left|s\right\rangle_3 \left|s\right\rangle_4 + \left|g\right\rangle_3 \left|g\right\rangle_4\right)/\sqrt{2}$. After the single photon passes through a beam splitter, the photon state can be written as $\left(\left|\uparrow\right\rangle + i\left|\downarrow\right\rangle\right)/\sqrt{2}$, where the photon $\left|\uparrow\right\rangle$ and $\left|\downarrow\right\rangle$ interacts with the qubit 2 and 3, respectively. The states can be written as

$$\left|\Psi\right\rangle_0 = \frac{\left|\uparrow\right\rangle + i\left|\downarrow\right\rangle}{\sqrt{2}} \otimes \frac{\left|s\right\rangle_1 \left|s\right\rangle_2 + \left|g\right\rangle_1 \left|g\right\rangle_2}{\sqrt{2}} \otimes \frac{\left|s\right\rangle_3 \left|s\right\rangle_4 + \left|g\right\rangle_3 \left|g\right\rangle_4}{\sqrt{2}}. \tag{S.30}$$

As with the two-node entanglement scheme, we can prepare the final state

$$\left|\Psi\right\rangle_f = \frac{\left|+i\right\rangle}{2}\left(\left|s\right\rangle_1 \left|s\right\rangle_2 \left|s\right\rangle_3 \left|s\right\rangle_4 - \left|g\right\rangle_1 \left|g\right\rangle_2 \left|g\right\rangle_3 \left|g\right\rangle_4\right) + \frac{\left|-i\right\rangle}{2}\left(\left|s\right\rangle_1 \left|s\right\rangle_2 \left|g\right\rangle_3 \left|g\right\rangle_4 - \left|g\right\rangle_1 \left|g\right\rangle_2 \left|s\right\rangle_3 \left|s\right\rangle_4\right), \tag{S.31}$$

which leads to the entangled state after detecting the single photon $\left|+i\right\rangle$ or $\left|-i\right\rangle$. To evaluate the effect of the expansion as a whole, we balance the fidelity and the successful probability that is $FP$, which is the fidelity without the post selection. Here we use a loose estimate, where we assume that the entangled state of two nodes is same and $f_{\mu=0} \approx -f_\mu$. It is easy to conclude that the performance is exponentially related to the number of nodes $N$, which can be written as $\left(FP\right)^{N-1}$ , and the fidelity $F$ and successful probability $P$ are the condition of two nodes.

## V. QUANTITATIVE ANALYSIS OF EXPERIMENTAL FEASIBILITY

We have discussed the the experimental feasibility qualitatively in the manuscript, and the quantum frequency conversion can be realized by the three-wave mixing process, the four-wave mixing process, as well as the optomechanical and Brillouin scattering interaction between light and mechanical vibrations.The choice of the choice of the specific implementation will depend on all kinds of factors, including the achievable cooperativities, the coherence times of

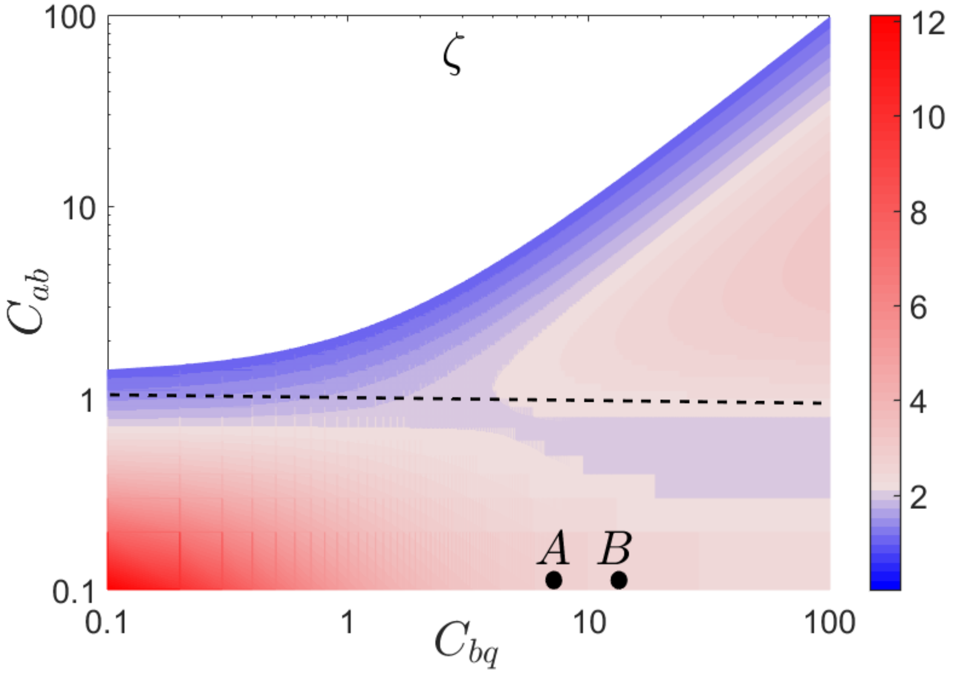


FIG. S5. The ratio $\zeta = F_{\mathrm{CQI}}P_{\mathrm{CQI}}/\left(F_{\mathrm{CAS}}P_{\mathrm{CAS}}\right)$ as the function of the cooperativity $C_{ab}\left(C_{bq}\right)$ for the two nodes with $\kappa_{b,o} = 4$ and other parameters are the same as in Fig. S2.

the qubits and intermediate modes, and the compatibility with existing quantum communication infrastructure. One promising experimental scheme involves a neutral atom as the qubit, with the target atomic transition at visible wavelengths. Although the thermal noise from intermediate modes can be ignored for this kind of experimental scheme, the CQI can also suppress the dephasing in addition to the decay of intermediate modes.

In Fig. S5, we plot the ratio $\zeta$ function of the cooperativity $C_{ab}\left(C_{bq}\right)$ for the two nodes, and the color area is corresponding to $\zeta > 1$, and the black line $C_{ab} = 1$ is the optimal conversion efficiency $\frac{\kappa_{a,ex}}{\kappa_a}\frac{\kappa_{b,ex}}{\kappa_b}$ for the cascaded scheme. The black dots correspond to the current experimental parameters (A dot [4, 5] and B dot [6]), whcih show the advantage over the traditional scheme. If we consider the thermal noise from the intermediate mode, the the overall advantage will be more obvious.

## VI. THE FIDELITY FOR THE INPUT PULSED LIGHT

In the previous discussion, the fidelity of the calculation was based on the stability of the system. In the actual physical system, we also need to consider the influence of input light with a certain line width on the fidelity, that is, the input light is pulsed. We assume that the input light is Gaussian pulsed light $f(t) \propto \exp(-t^2/\tau^2)$, where $\tau$ is the pulse length of the input light.The corresponding fidelity can be rewritten as

$$F = \frac{\int_0^\tau \left|f_{\mu=0} - f_\mu\right|^2 dt}{\int_0^\tau 2\left(\left|f_{\mu=0}\right|^2 + \left|f_\mu\right|^2\right) dt}. \tag{S.32}$$

The corresponding fidelity for the CQI is shown in Fig. S6 with the diffrent decay rates $\kappa_{b,o} = 10,\ 4,\ 0.1$. As the pulse length increases gradually, the fidelity becomes closer to the steady-state results. The time to steady state is basically independent of the intermediate mode dissipation, and is determined by the time required for the stability

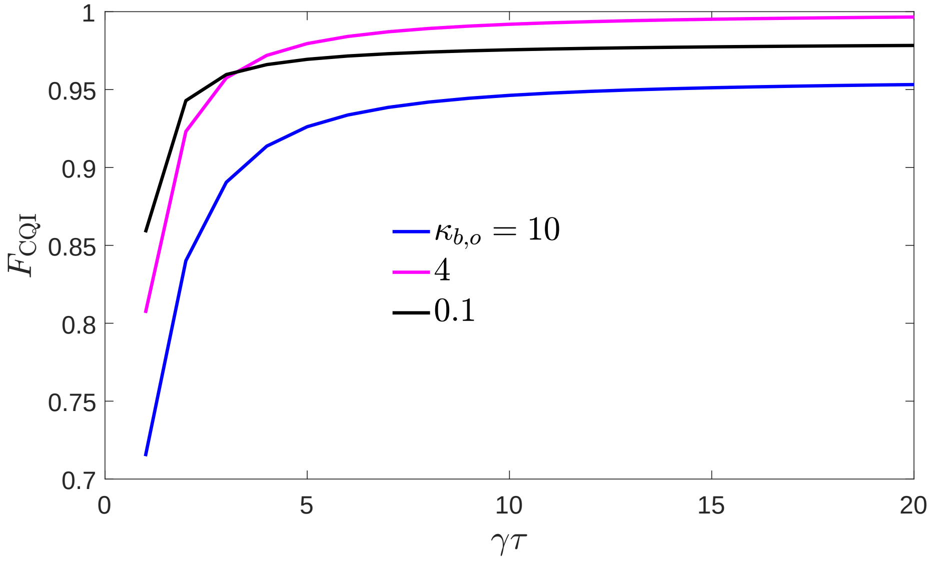


FIG. S6. The fidelity $F_{\rm CQI}$ as the function of the pulse length $\tau$ for the two nodes with $\kappa_{b,o} = 10$, 4, 0.1 and other parameters are the same as in Fig. S2.

of the system.


[1] J.-T. Shen and S. Fan, Coherent single photon transport in a one-dimensional waveguide coupled with superconducting quantum bits, Physical Review letters **95**, 213001 (2005).
[2] S. Rosenblum, A. Borne, and B. Dayan, Analysis of deterministic swapping of photonic and atomic states through single-photon raman interaction, Physical Review A **95**, 033814 (2017).
[3] C.-H. Yan, M. Li, X.-B. Xu, Y.-L. Zhang, X.-Y. Ma, and C.-L. Zou, Unidirectional propagation of single photons realized by a scatterer coupled to whispering-gallery-mode microresonators, Physical Review A **107**, 033713 (2023).
[4] T. Tiecke, J. D. Thompson, N. P. de Leon, L. Liu, V. Vuletić, and M. D. Lukin, Nanophotonic quantum phase switch with a single atom, Nature **508**, 241 (2014).
[5] I. Shomroni, S. Rosenblum, Y. Lovsky, O. Bechler, G. Guendelman, and B. Dayan, All-optical routing of single photons by a one-atom switch controlled by a single photon, Science **345**, 903 (2014).
[6] M. Scheucher, A. Hilico, E. Will, J. Volz, and A. Rauschenbeutel, Quantum optical circulator controlled by a single chirally coupled atom, Science **354**, 1577 (2016).
